# Supplementary material for: Finite Membrane Thickness Influences Hydrodynamics on the Nanoscale
Source: arXiv:2505.05776 ancillary file (2025-08-28)
Supplement: Supplementary file 1 [file QuiscentArticle_SI.pdf]

# Supplementary Material

## Finite Membrane Thickness Influences Hydrodynamics on the Nanoscale

Zachary G. Lipel[1,3‡] ,Yannick A. D. Omar[1,2,§] , Dimitrios Fraggedakis[3,*] ,

[1] Department of Chemical & Biomolecular Engineering, University of California, Berkeley, CA 94720, USA
[2] Department of Chemical Engineering, Massachusetts Institute of Technology, Massachusetts 02139, USA
[3] Department of Chemical and Biological Engineering, Princeton University, Princeton, NJ 08544

# Contents

**1 Curvilinear geometry** **1**
1.1 Euclidean three-dimensional space . . . . . . . . . . . . . . . . . . . . . . . . . . . . 2
1.2 Geometry and kinematics of the bilayer . . . . . . . . . . . . . . . . . . . . . . . . . 3

**2 Governing equations** **4**

**3 Dimensionless parameters** **7**

**4 Perturbation analysis** **7**
4.1 The general unperturbed equations . . . . . . . . . . . . . . . . . . . . . . . . . . . . 8
4.2 The general perturbed equations . . . . . . . . . . . . . . . . . . . . . . . . . . . . . 9

**5 Problem solution** **10**
5.1 Membrane parametrization and base state . . . . . . . . . . . . . . . . . . . . . . . . 11
5.2 The perturbed equations . . . . . . . . . . . . . . . . . . . . . . . . . . . . . . . . . . 11
5.3 Linear response solution for finite thickness membranes . . . . . . . . . . . . . . . . . 12

**6 Dispersion relation and hydrodynamics** **14**
6.1 Dispersion relation . . . . . . . . . . . . . . . . . . . . . . . . . . . . . . . . . . . . . 14
6.2 Induced flow fields for single modes . . . . . . . . . . . . . . . . . . . . . . . . . . . . 15
6.3 The emergence of flow reversal . . . . . . . . . . . . . . . . . . . . . . . . . . . . . . 18

**7 Comparison with intermonolayer slip theories** **19**

**Supporting References** **21**

# 1 Curvilinear geometry

Lipid bilayers can undergo arbitrarily large deformations [1, 2], motivating the use of curvilinear coordinates in their mathematical description. In the following, we revisit the use of differential geometry for coordinate systems in two and three dimensions.

‡zl4808@princeton.edu
§yadomar@mit.edu
*dimfraged@gmail.com & dfrag@princeton.edu

### 1.1 Euclidean three-dimensional space

Consider a point in three-dimensional Euclidean space with Cartesian coordinates $x^i$ (for $i = 1, 2, 3$), as depicted in Fig. 1, where we use Latin indices to span the set $\{1, 2, 3\}$. We introduce a local, arbitrary (real) curvilinear parametrization $\zeta^i$

$$x^i = x^i(\zeta^1, \zeta^2, \zeta^3), \qquad \det\left(\frac{\partial x^i}{\partial \zeta^j}\right) \neq 0 \ . \tag{1}$$

which ensures the existence of a unique inverse of the preceding transformation. The parametrization $\{\zeta^i\}$ defines a set of tangent basis vectors, $\boldsymbol{g}_i := \partial_i \boldsymbol{x}$, that span the tangent space at $\boldsymbol{x}$. Any three-dimensional vector $\boldsymbol{u} \in \mathbb{R}^3$ can be expressed in terms of $\{\boldsymbol{g}_i\}$ as $\boldsymbol{u} = u^i \boldsymbol{g}_i$, where here and henceforth, we use Einstein summation convention.

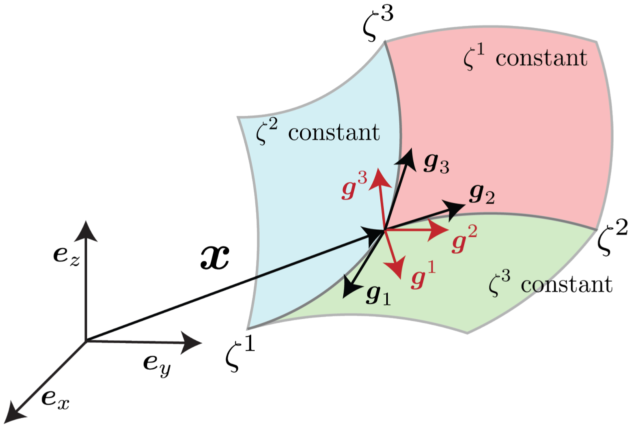


Figure 1: Local geometry of a point in three-dimensional Euclidean space.

Based on the parametrization of Eq. (1), we can express the first fundamental form as $ds^2 = d\boldsymbol{x} \cdot d\boldsymbol{x} = \boldsymbol{g}_i \cdot \boldsymbol{g}_j d\theta^i d\theta^j$ [3,4]. This motivates the definition of the covariant metric, $g_{ij} := \boldsymbol{g}_i \cdot \boldsymbol{g}_j$, which characterizes the metric properties of the tangent space in the curvilinear system. Furthermore, we introduce the reciprocal basis $\boldsymbol{g}^i = \epsilon^{ijk} \boldsymbol{g}_j \times \boldsymbol{g}_k / \left((\boldsymbol{g}_1 \times \boldsymbol{g}_2) \cdot \boldsymbol{g}_3\right)$, where $\epsilon^{ijk}$ is the unit permutator. This definition yields $\boldsymbol{g}^i \cdot \boldsymbol{g}_j = \delta^i_j$, and the reciprocal space metric, $g^{ij} := \boldsymbol{g}^i \cdot \boldsymbol{g}^j$, that satisfies $g_{ij} g^{jk} = \delta^k_i$. As a result, the tangent and reciprocal space metric tensors can be used to raise and lower indices through the relations $\boldsymbol{g}_i = g_{ij} \boldsymbol{g}^j$ and $\boldsymbol{g}^i = g^{ij} \boldsymbol{g}_j$. Therefore, $\boldsymbol{u} = u^i \boldsymbol{g}_i = u^i g_{ij} \boldsymbol{g}^j = u_j \boldsymbol{g}^j$, where we see that the components in each basis are related by $u^i = g^{ij} u_j$, and similarly, $u_i = g_{ij} u^j$.

The covariant derivative with respect to $\zeta^i$, $(\cdot)|_i$, represents how a quantity changes along the $\zeta^i$ direction while accounting for the dependence of the local tangent basis on that direction. For instance, the covariant derivative of vector components $u^j$ along $\zeta^i$ is expressed as $u^i|_j = u^i_{,j} + u^k \Gamma^i_{kj}$, where $\Gamma^i_{kj} := \frac{1}{2} g^{in} \left(g_{nj,k} + g_{nk,j} - g_{kj,n}\right)$ is the Christoffel symbol of the second kind, which accounts for the variation of the coordinate basis and ensures that differentiation is performed consistently within a curved space.

The formalism of differential geometry allows us to describe arbitrarily large, local deformations of lipid bilayers. In the following section, we will reiterate the main results of Refs. [5–7], which employ differential geometry and dimension reduction to arrive at an effectively two-dimensional theory explicit in the membrane thickness.

## 1.2 Geometry and kinematics of the bilayer

We model the lipid bilayer as a three-dimensional body, denoted as $\mathcal{M}$. This body is situated within bulk media $\mathcal{B}_{\pm}$ and bounded by surfaces $\mathcal{S}^{\pm}$, with the mid-surface denoted by $\mathcal{S}_0$, as depicted in Fig. 2–(a). For our parametrization, we select in-plane coordinates $\{\theta^1, \theta^2\}$. On the mid-surface $\mathcal{S}_0$, a point $\boldsymbol{x}_0 \in \mathcal{S}_0$ can be expressed as $\boldsymbol{x}_0(\theta^1, \theta^2, t)$. From this point onward, Greek indices span the set $\{1, 2\}$. The parametrization $\{\theta^\alpha\}$ naturally gives rise to the tangent basis vectors $\boldsymbol{a}_\alpha := \partial_\alpha \boldsymbol{x}_0$, which span the tangent space to the mid-surface $\mathcal{S}_0$. The normal to the mid-surface is denoted by $\boldsymbol{n} = \boldsymbol{a}_1 \times \boldsymbol{a}_2 / |\boldsymbol{a}_1 \times \boldsymbol{a}_2|$, and together the in-plane tangent and normal vectors form a basis in $\mathbb{R}^3$. Therefore, any three-dimensional vector $\boldsymbol{u}$ can be expressed in terms of $\{\boldsymbol{a}_\alpha, \boldsymbol{n}\}$, i.e., $\boldsymbol{u} = u^\alpha \boldsymbol{a}_\alpha + u\boldsymbol{n}$. It is worth noting that these components can differ from the three dimensional basis components introduced in Eq. (1), $\{u_i\}$, where $i$ refers to a distinct parametrization defined anywhere in the system rather than restricted to the membrane. In general, the notation will be clear from the context. The reciprocal basis is defined in a similar manner as discussed in Sec. 1.1 with $\boldsymbol{a}^\alpha = \epsilon^{\alpha\gamma} \boldsymbol{a}_\gamma \times \boldsymbol{n} / [\boldsymbol{a}_1, \boldsymbol{a}_2, \boldsymbol{n}]$, where $\epsilon^{\alpha\gamma}$ is the two-dimensional unit permutator [3].

We define the surface covariant metric as $a_{\alpha\beta} := \boldsymbol{a}_\alpha \cdot \boldsymbol{a}_\beta$, serving as a measure of distances on the mid-surface. Similar to the three dimensional case, its inverse is defined by $a^{\alpha\beta} a_{\beta\gamma} = \delta^\alpha_\gamma$, and we can utilize both to raise and lower indices, for example, $u_\beta = a_{\beta\alpha} u^\alpha$ and $u^\beta = a^{\beta\alpha} u_\alpha$. The curvature tensor, $\mathbf{b}$, has components defined by $b_{\alpha\beta} := \boldsymbol{n} \cdot \boldsymbol{x}_{0,\alpha\beta}$. Its trace $2H := \mathrm{Tr}\ \mathbf{b}$ and determinant $K := \det \boldsymbol{b}$ correspond to the mean and Gaussian curvatures, respectively.

The covariant derivative with respect to the mid-surface parametrization $\{\theta^\alpha\}$ is denoted as $(\cdot)_{:\alpha}$ for vectorial quantities and $(\cdot)_{;\alpha}$ for tensorial quantities. For instance, the covariant derivative of vector components $u^\beta$ along $\theta^\alpha$ is expressed as $u^\beta_{:\alpha} = u^\beta_{,\alpha} + u^\gamma \Gamma^\beta_{\gamma\alpha}$, where

$$\Gamma^\beta_{\gamma\alpha} := \frac{1}{2} a^{\beta\mu} \left( a_{\mu\alpha,\gamma} + a_{\mu\gamma,\alpha} - a_{\gamma\alpha,\mu} \right) \tag{2}$$

is the Christoffel symbol of the second kind.

While we account for membrane thickness, our approach assumes $\delta \ll L_c$, where $L_c$ is a characteristic in-plane length scale, such as the radius of curvature of a cellular membrane. Under this condition, we additionally invoke the classical Kirchhoff–Love (K-L) kinematic assumption, which assumes that material lines remain straight and normal to the mid-surface during deformation. This condition allows a one-to-one mapping from the mid-surface to any point within the

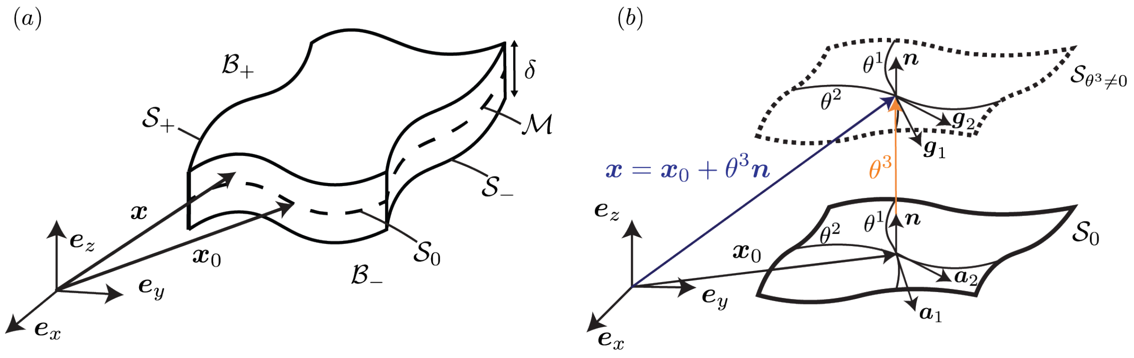


Figure 2: (a) Membrane and its bounding surfaces embedded in Euclidean 3-space. (b) Local parametrization of the mid-surface $\mathcal{S}_0$. Contravariant basis vectors are not shown explicitly.

membrane thickness.

Following Refs. [5, 6], the membrane position vector satisfies the ansatz

$$\boldsymbol{x} = \boldsymbol{x}_0 + \theta^3 \boldsymbol{n} \ , \tag{3}$$

where $\theta^3 \in [-\delta/2, \delta/2]$ parameterizes the thickness direction, and the mid-surface corresponds to $\theta^3 = 0$ (see Fig. 2–(b)). From Eq. (3), the membrane's local covariant basis can be expressed in terms of the mid-surface geometry as $\boldsymbol{g}_\alpha = \boldsymbol{a}_\alpha - \theta^3 b_\alpha^\beta \boldsymbol{a}_\beta$ and $\boldsymbol{g}^\alpha = \boldsymbol{a}^\alpha + \frac{1}{2}\theta^3 b_\beta^\alpha \boldsymbol{a}^\beta + \mathcal{O}(|\delta \boldsymbol{b}|^2)$. A more complete expression for the reciprocal basis is given in Ref. [6].

An admissible velocity field can be derived from Eq. (3) under the K-L constraint [6]. Since $\theta^3$ is constant along particle trajectories, i.e., $\frac{\mathrm{d}\theta^3}{\mathrm{d}t} = 0$, we may differentiate Eq. (3) to obtain

$$\boldsymbol{v} = \frac{\mathrm{d}}{\mathrm{d}t}\boldsymbol{x} = \boldsymbol{v}_0(\theta^\alpha, t) - \theta^3 \dot{\boldsymbol{n}} = \boldsymbol{v}_0(\theta^\alpha, t) + \theta^3 \left( v_{,\gamma} + v_0^\beta b_{\beta\gamma} \right) a^{\gamma\alpha} \boldsymbol{a}_\alpha \ , \tag{4}$$

where $\boldsymbol{v}_0 = v_0^\alpha \boldsymbol{a}_\alpha + v\boldsymbol{n}$ is the mid-surface velocity, and we have used the result [6]

$$\frac{\mathrm{d}}{\mathrm{d}t}\boldsymbol{n} = -\left( v_{,\gamma} + v_0^\beta b_{\beta\gamma} \right) a^{\gamma\alpha} \boldsymbol{a}_\alpha \ . \tag{5}$$

This form of the velocity field reflects the fact that, under the K-L constraint, both $\boldsymbol{v}$ and other membrane quantities such as stress and density admit well-defined polynomial expansions in $\theta^3$. Notably, Eq. (4) shows that in-plane surface motions can exist even when $\boldsymbol{v}_0 = 0$, a feature not present in strict surface theories. These expansions are central to the $(2+\delta)$-dimensional theory developed in Refs. [5–7]. In Section 2, we summarize this framework and present the resulting reduced equations of motion.

## 2 Governing equations

In this section, we adopt the $(2+\delta)$-dimensional framework developed in Refs. [5–7] and summarize the equations of motion for mid-surface incompressible lipid bilayers. The $(2+\delta)$-dimensional framework provides an effectively two-dimensional description by employing a spectral decomposition of the membrane quantities such as position $\boldsymbol{x}$, velocity $\boldsymbol{v}$, and stress $\boldsymbol{\sigma}$. Additionally, we use Stokes equations to model the bulk fluid flow of the membrane surroundings. Finaly, we write the boundary conditions governing membrane-bulk interactions and the far-field flow behavior.

We start by representing the membrane fields using spectral expansions in the thickness direction

$$\boldsymbol{x}(\theta^\alpha, \theta^3, t) = \sum_{k=0}^{1} \boldsymbol{x}_k(\theta^\alpha, t) P_k[\Theta(\theta^3)] \ , \tag{6a}$$

$$\boldsymbol{v}(\theta^\alpha, \theta^3, t) = \sum_{k=0}^{1} \boldsymbol{v}_k(\theta^\alpha, t) P_k[\Theta(\theta^3)] \ , \tag{6b}$$

$$\boldsymbol{\sigma}(\theta^\alpha, \theta^3, t) = \sum_{k=0}^{\infty} \boldsymbol{\sigma}_k(\theta^\alpha, t) P_k[\Theta(\theta^3)] \ , \tag{6c}$$

$$\rho(\theta^\alpha, \theta^3, t) = \sum_{k=0}^{\infty} \rho_k(\theta^\alpha, t) P_k[\Theta(\theta^3)] \ . \tag{6d}$$

Here, $\boldsymbol{\sigma}$ and $\rho$ are the membrane stress tensor and density, respectively. The function $\Theta$ maps $\Theta : [-\delta/2, \delta/2] \to [-1, 1]$, and $\{P_k[\theta]\}$ is a set of complete orthogonal polynomials defined in $\theta \in [-1, 1]$. Here, we choose $\{P_k[\theta]\}$ from the family of Chebyshev polynomials due to their analytical and computational tractability [8].

Next, we outline the order-of-magnitude assumptions required to truncate the expansions in Eqs. (6). As detailed in Ref. [6], these assumptions ensure analytically tractable equations while preserving the essential physics of finite-thickness membranes. First, we assume that key physical quantities, such as bending forces and moments, vary over length scales $L$ much greater than the membrane thickness $\delta$. In addition, we consider that the bilayer curvature remains small [6], i.e.,

$$(\delta H)^2 \ll 1 \quad \& \quad \delta^2 |K| \ll 1 \ . \tag{7}$$

Given that $\delta \sim \mathcal{O}(1)$ nm for biological membranes, this condition is generally satisfied in the regime where $L \sim H^{-1} \gg \delta$ [9–12]. Additionally, we introduce the following characteristic in-plane length scales $\ell_c$, $\ell_v$, $\ell_s$ governing curvature, velocity, and stress variations, respectively. We assume that the curvature does not vary significantly over scales much smaller than the stress distribution, i.e., $\ell_c \not\ll \ell_s$, and that both satisfy

$$\left(\frac{\delta}{\ell_c}\right)^2 \ll 1 \quad \& \quad \left(\frac{\delta}{\ell_s}\right)^2 \ll 1 \ . \tag{8}$$

Furthermore, we assume that the first-order in-plane velocity coefficient is small relative to the zeroth-order coefficient, i.e.

$$v_1^\alpha \ll v_0^\alpha \ . \tag{9}$$

Similarly, for the in-plane stresses, we assume that higher-order coefficients $\sigma_k^{\alpha\beta}$ $(k \geq 2)$ are at most comparable in magnitude to the zeroth- and first-order terms. This allows us to systematically neglect higher-order terms using the length-scale assumptions in Eqs. (7) and (8). Additional details on these approximations can be found in Ref. [6]. With these assumptions in place, we now proceed to discuss the equations of motion.

We first connect the expansions for the position and velocity, Eqs. (6a) and (6b), to the results in Sec. 1.2. Recall the membrane position takes the form given in Eq. (3). Upon comparison with Eq. (6a), we find that

$$\boldsymbol{x}_1 = \frac{\delta}{2}\boldsymbol{n} \ , \tag{10}$$

Similarly, Eq. (4) implies that the velocity has a first-order expansion $\boldsymbol{v} = \boldsymbol{v}_0 + \boldsymbol{v}_1 P_1[\Theta]$, where

$$\boldsymbol{v}_0 = v_0^\alpha(\theta^\alpha, t)\boldsymbol{a}_\alpha + v(\theta^\alpha, t)\boldsymbol{n} \ , \tag{11}$$

$$\boldsymbol{v}_1(\theta^\alpha, t) = -\frac{\delta}{2}\left(v_{,\gamma} + v_0^\beta b_{\beta\gamma}\right) a^{\gamma\alpha}\boldsymbol{a}_\alpha \ . \tag{12}$$

This leads to the observation that $\boldsymbol{v}_1 \cdot \boldsymbol{n} = v_1^3 = 0$, which is a result of the constraint that the thickness is independent of time.

With the above formulation, Refs. [6, 7] show that for a mid-surface incompressible membrane immersed in a viscous medium, the governing equations for the in-plane and out-of-plane linear momentum balances and the continuity equation are respectively given by

$$0 = \lambda_{,\alpha} + \frac{k_{\mathrm{b}}}{2}K^{,\alpha} + 2\mu^{\mathrm{m}}\left(d^{\alpha\beta}_{:\beta} - v_{,\beta}b^{\alpha\beta} - 2vH^{,\alpha}\right) + \frac{\delta}{2}(b^\alpha_\lambda - 2\delta^\alpha_\lambda H)\,[\![t^\alpha_{\mathrm{visc}}]\!] + 2\,\langle t^\alpha_{\mathrm{visc}}\rangle \ , \tag{13a}$$

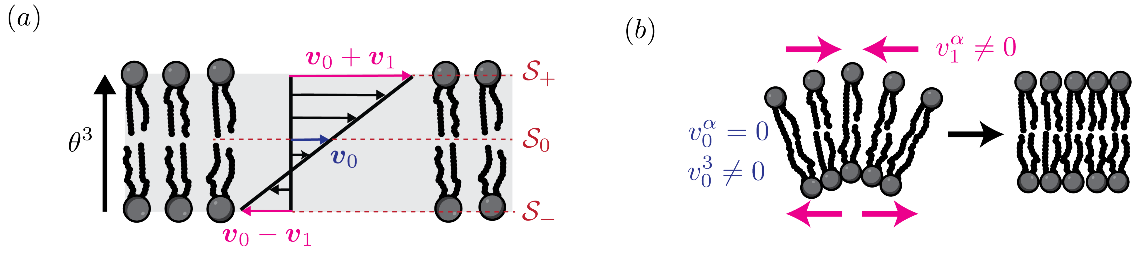


Figure 3: (a) Schematic of lipid in-plane flows. The velocity varies linearly with the thickness direction. (b) Deformation where surface motion is possible without in-plane motion.

$$
\begin{aligned}
0 &= 2H\left(\lambda + \delta\left\langle p\right\rangle\right) - k_{\mathrm{b}} H(4H^2 - 3K) - k_{\mathrm{b}}\Delta_s H + 2\mu^{\mathrm{m}}\left(d^{\alpha\beta} b_{\alpha\beta} - v(4H^2 - 2K)\right) \\
&\quad + \frac{\delta}{2}\left[\!\left[ t^\alpha_{\mathrm{visc}} \right]\!\right]_{:\alpha} - \left[\!\left[ p \right]\!\right] + 2\left\langle t^n_{\mathrm{visc}} \right\rangle \ , \qquad (13\mathrm{b}) \\
0 &= v^\alpha_{:\alpha} - 2vH \ , \qquad (13\mathrm{c})
\end{aligned}
$$

where $\lambda$ is the membrane tension, $k_{\mathrm{b}}$ is the membrane bending modulus, and $\mu^{\mathrm{m}}$ is the membrane viscosity. The double bracket notation, $\left[\!\left[\cdot\right]\!\right] \coloneqq (\cdot)^+ - (\cdot)^-$, represents the jump in quantities evaluated at the membrane surfaces, $\mathcal{S}_\pm$, while the angled bracket notation, $2\left\langle\cdot\right\rangle \coloneqq (\cdot)^+ + (\cdot)^-$, indicates their average. The surface Laplacian operating on the curvature $H$ is defined as $\Delta_s(\cdot) \coloneqq (\cdot)_{:\alpha\beta}a^{\alpha\beta}$ [3]. The bulk viscous tractions acting on the membrane surfaces are characterized by the in-plane components, $t^\alpha_{\mathrm{visc}}$, and normal components, $t^n_{\mathrm{visc}}$, while the bulk incompressibility introduces a pressure term, $p$. Finally, $d^{\alpha\beta} = \frac{1}{2}\left(v_0^{\alpha:\beta} + v_0^{\beta:\alpha}\right)$ denotes the in-plane strain rate at the mid-surface.

In addition to the membrane equations, we require a description of the bulk medium dynamics. In the context of biological membranes, inertia is negligible so that the bulk fluid velocity $\boldsymbol{u}$ and pressure $p$ are governed by the Stokes equations and continuity, i.e.

$$
\begin{aligned}
-\nabla p_\pm + \mu^{\mathrm{b}}\nabla^2 \boldsymbol{u}_\pm &= 0 \ , \qquad (14\mathrm{a}) \\
\nabla\cdot\boldsymbol{u}_\pm &= 0 \ , \qquad (14\mathrm{b})
\end{aligned}
$$

where $\mu^{\mathrm{b}}$ is the bulk viscosity and $\pm$ refers to the domains located at the top and bottom of the membrane, respectively.

Finally, we require a set of boundary conditions in order to close the problem. We assume that at infinity, the bulk fluid is at rest, leading to the following conditions for the velocities and pressure

$$
\begin{aligned}
\boldsymbol{u}_\pm\Big|_{z\to\pm\infty} &= 0 \ , \qquad (15\mathrm{a}) \\
p_\pm\Big|_{z\to\pm\infty} &= \ \mathrm{const.} \qquad (15\mathrm{b})
\end{aligned}
$$

We will consider the case in which the pressure constant in Eq. (15b) is the same on either side of the membrane, consistent with the initial condition that the membrane is flat. Without loss of generality, we set this constant to zero. Additionally, at the membrane-fluid interfaces, in-plane and out-of-plane no-slip conditions between the bilayer and the bulk yield

$$
u^\alpha_\pm = v^\alpha \mp \frac{\delta}{2}\left(v^{,\alpha} + b^\alpha_\beta v^\beta\right) \ , \qquad (16\mathrm{a})
$$

$$u^n_\pm = v^n \;, \tag{16b}$$

where we have used the kinematics, Eqs. 3 and 4, to evaluate the membrane velocity at the bounding surfaces [6, 7].

# 3 Dimensionless parameters

We seek a set of non-dimensional groupings governing the present physics. To this end, we scale all lengths with the typical system size, $L$, the tension with the base state tension $\Lambda$, the velocity with $U$, and the time with $\tau = L/U$. In what follows, we denote dimensionless quantities with an asterisk, $(\cdot)^*$. The Stokes equations in terms of non-dimensional quantities are

$$-\nabla^* p^*_\pm + \nabla^{*2} \boldsymbol{u}^*_\pm = 0 \;, \tag{17a}$$

$$\nabla^* \cdot \boldsymbol{u}^*_\pm = 0 \;, \tag{17b}$$

where we chose the bulk pressure scale as $p_c := \mu^{\mathrm{b}} U/L$ [3, 13].

Application of the Buckingham $\pi$ theorem shows that we can express the membrane equations in terms of four dimensionless numbers. The resulting dimensionless numbers are the Föppl-von Kármán number [14], $\Gamma := \Lambda L^2/k_{\mathrm{b}}$ comparing membrane tension to bending forces, the Scriven-Love number $\mathrm{SL} := \mu^{\mathrm{m}} V L/k_{\mathrm{b}}$ [15] relating membrane viscous to bending forces, and the capillary number $\mathrm{Ca} := \mu^{\mathrm{b}} U/\Lambda$ contrasting bulk viscous forces to membrane tension. As the last dimensionless group, we choose the ratio between the membrane thickness $\delta$ and the characteristic length scale $L$, i.e. $\ell := \delta/L$, which characterizes finite thickness effects. With these definitions, the non-dimensional form of the membrane equations reads:

$$0 = \lambda^{*,\alpha} + \frac{1}{2\Gamma} K^{*,\alpha} + 2\frac{\mathrm{SL}}{\Gamma}\left(d^{*\alpha\beta}_{:\beta} - v^*_{,\beta} b^{*\alpha\beta} - 2v^* H^{*,\alpha}\right) + \mathrm{Ca}\left(\frac{\ell}{2}(b^{*\alpha}_{\lambda} - 2\delta^\alpha_\lambda H^*)\,[\![ t^{*\alpha}_{\mathrm{visc}} ]\!] + 2\,\langle t^{*\alpha}_{\mathrm{visc}}\rangle\right) , \tag{18a}$$

$$\begin{aligned} 0 = {} & 2H^*\left(\lambda^* + \ell\,\langle p^*\rangle\right) - \frac{1}{\Gamma} H^*(4H^{*2} - 3K^*) - \frac{1}{\Gamma}\Delta_s H^* + 2\frac{\mathrm{SL}}{\Gamma}\left(d^{*\alpha\beta} b^*_{\alpha\beta} - v^*(4H^{*2} - 2K^*)\right) \\ & + \mathrm{Ca}\left(\frac{\ell}{2}\,[\![ t^{*\alpha}_{\mathrm{visc}} ]\!]_{:\alpha} - [\![ p^* ]\!] + 2\,\langle t^{*n}_{\mathrm{visc}}\rangle\right) , \end{aligned} \tag{18b}$$

$$0 = v^\alpha_{:\alpha} - 2vH \;. \tag{18c}$$

Note that for $\ell \to 0$, we recover the classical two-dimensional membrane equations [15] up to nonlinear terms. However, it is possible for finite thickness effects to contribute to membrane dynamics when $\mathrm{Ca}\ell \sim O(1/\delta)$. This may be the case when the membrane is under the presence of a strong shear and/or extensional flow fields. We will omit the $(\cdot)^*$ superscript for the ease of notation and consider all quantities to be dimensionless, unless otherwise noted.

# 4 Perturbation analysis

In this section, we derive the base and perturbed state equations for nearly flat membranes. These equations allow us to study thermal fluctuations of large vesicles and other small curvature geometries using linear response theory. In the following, base state and perturbed quantities will be denoted by the scripts (0) and (1), respectively.

### 4.1 The general unperturbed equations

In this section, we will derive the general unperturbed equations for a base state where the membrane is flat. We choose a Cartesian parametrization: $\{\theta^1, \theta^2, \theta^3\} = \{x, y, z\}$. This choice allows us to express a point on the mid-surface $\boldsymbol{x}^{\mathrm{mid}}_{(0)} \in \mathcal{S}_0$ as

$$\boldsymbol{x}^{\mathrm{mid}}_{(0)} = x\boldsymbol{e}_x + y\boldsymbol{e}_y \ , \tag{19}$$

where the set $\{\boldsymbol{e}_i\}$ are Cartesian basis vectors. Using the results from Sec. 1.2, Eq. (19) yields the following relationships:

$$\begin{aligned} &\boldsymbol{a}^{(0)}_\alpha = \boldsymbol{e}_\alpha \ , \quad a^{(0)}_{\alpha\beta} = \delta_{\alpha\beta} \ , \quad a^{\alpha\beta}_{(0)} = \delta^{\alpha\beta} \ , \quad \boldsymbol{n}_{(0)} = \boldsymbol{e}_z \ , \\ &b^{(0)}_{\alpha\beta} = 0 \ , \quad H_{(0)} = 0 \ , \quad K_{(0)} = 0 \ , \quad \text{and} \quad \Gamma^{\alpha \ (0)}_{\lambda\mu} = 0 \ . \end{aligned} \tag{20}$$

We note here that the metric tensor is the identity tensor. As a result, the reciprocal basis is equivalent to the covariant basis. Therefore, we assume that repeated indices are summed over, even if they both appear as sub- or superscripts (e.g. $u^\beta_{,\alpha\alpha} = u^{\beta,\alpha}_{,\alpha} = u^\beta_{,xx} + u^\beta_{,yy}$). Next, we write the membrane base state velocity as

$$\boldsymbol{v}_{(0)} = v^\alpha_{(0)}\boldsymbol{a}_\alpha + v^3_{(0)}\boldsymbol{n} \tag{21}$$

$$= v^\alpha_{(0)}\boldsymbol{e}_\alpha + v^z_{(0)}\boldsymbol{e}_z \tag{22}$$

$$= v^\alpha_{(0)}\boldsymbol{a}^\alpha \ , \tag{23}$$

where $v^z_{(0)}$ is zero since the membrane is assumed flat and therefore moves at most in the in-plane directions. Similarly, the bulk unperturbed velocities are

$$\boldsymbol{u}_{\pm,(0)} = u^i_{\pm,(0)}\boldsymbol{e}_i \ , \tag{24}$$

The in-plane surface tractions $t^\alpha_\pm = \boldsymbol{t}_\pm \cdot \boldsymbol{a}^\alpha$ are then

$$t^\alpha_{(0)\pm} = \pm\left(u^z_{(0),\alpha} + u^\alpha_{(0),z}\right) \ , \tag{25}$$

and the normal components $t^n_\pm = \boldsymbol{t}_\pm \cdot \boldsymbol{n}$ become

$$t^n_{(0)} = -p_{(0)} + 2\mu^{\mathrm{b}}u^z_{(0),z} \ . \tag{26}$$

The jumps and averages of the applied tractions in the base state can then be written as

$$\left[\!\left[t^\alpha_{(0)}\right]\!\right] = 2\left\langle u^z_{(0),\alpha} + u^\alpha_{(0),z}\right\rangle \ , \tag{27}$$

$$2\left\langle t^\alpha_{(0)}\right\rangle = \left[\!\left[u^z_{(0),\alpha} + u^\alpha_{(0),z}\right]\!\right] \ , \tag{28}$$

$$\left[\!\left[t^n_{(0)}\right]\!\right] = -\left[\!\left[p_{(0)}\right]\!\right] + 2\left[\!\left[u^z_{(0),z}\right]\!\right] \ , \tag{29}$$

$$\left\langle t^n_{(0)}\right\rangle = -\left\langle p_{(0)}\right\rangle + 2\left\langle u^z_{(0),z}\right\rangle \ . \tag{30}$$

We now proceed to derive the unperturbed equations of motion. The membrane continuity equation, Eq. (13c), becomes

$$v^\alpha_{(0),\alpha} = 0 \ . \tag{31}$$

The shape equation, Eq. (13b), reads

$$0 = -\left[\!\left[p_{(0)}\right]\!\right] + \ell \left\langle u^z_{(0),\alpha} + u^\alpha_{(0),z} \right\rangle_{,\alpha} + 2\left[\!\left[u^z_{(0),z}\right]\!\right] \ , \tag{32}$$

and the in-plane equations, Eq. (13a), are

$$0 = \lambda_{(0),\beta} a^{\alpha\beta} + \frac{\mathrm{SL}}{\Gamma} v^\alpha_{(0),\beta\beta} + \mathrm{Ca}\Big( \left[\!\left[u^z_{(0),\alpha} + u^\alpha_{(0),z}\right]\!\right] - \ell \left\langle p_{(0)} \right\rangle_{,\beta} a^{\alpha\beta} \Big) \ , \tag{33}$$

where we employed the membrane continuity equation, Eq. (31). The bulk base state continuity equation reads

$$u^i_{(0),i} = 0 \ , \tag{34}$$

and the Stokes equations are

$$0 = -p_{(0),i} + (u^i_{(0),jj}) \ . \tag{35}$$

Equations (31)–(35) represent the general unperturbed equations for a planar geometry. We will now consider small perturbations around this base state.

## 4.2 The general perturbed equations

Let us consider the general perturbed equations. Due to thermal fluctuations, the membrane shape undulates and experiences shape deformations. In this case, we can express the mid-surface in terms of a height field quantifying its displacement from $z = 0$, i.e.

$$\boldsymbol{x}_0 = \boldsymbol{x}^{\mathrm{mid}}_{(0)} + \epsilon h(x, y, t) \boldsymbol{e}_z \ , \tag{36}$$

where $\epsilon \ll 1$ is the perturbation parameter. To first order in $\epsilon$, we now find

$$\begin{aligned} &\boldsymbol{a}_\alpha = \boldsymbol{e}_\alpha + \epsilon\ h_{,\alpha} \boldsymbol{e}_z \ , \quad a_{\alpha\beta} = \delta_{\alpha\beta} \ , \quad a^{\alpha\beta} = \delta^{\alpha\beta} \ , \quad \boldsymbol{n} = \boldsymbol{e}_z - \epsilon h_{,\alpha} \boldsymbol{e}_\alpha \ , \\ &b_{\alpha\beta} = \epsilon h_{,\alpha\beta} \ , \quad H = \epsilon \frac{1}{2} \Delta_s h \ , \quad K = 0 \ , \quad \text{and} \quad \Gamma^\alpha_{\lambda\mu} = 0 \ . \end{aligned} \tag{37}$$

The membrane velocity and effective surface tension become

$$v^\alpha = v^\alpha_{(0)} + \epsilon v^\alpha_{(1)} \ , \quad v = \epsilon h_{,t} \ , \quad \lambda = \lambda_{(0)} + \epsilon \lambda_{(1)} \ . \tag{38}$$

Similarly, we have for the bulk velocities

$$\boldsymbol{u} = \left( u^i_{(0)} + \epsilon u^i_{(1)} \right) \boldsymbol{e}_i \ . \tag{39}$$

The $\mathcal{O}(\epsilon)$ membrane continuity equation becomes

$$v^\alpha_{(1),\alpha} = 0 \ . \tag{40}$$

In order to evaluate the contributions from the bulk tractions acting on the membrane, we calculate the following

$$\boldsymbol{e}_i \cdot \boldsymbol{a}_\alpha = \delta_{i\alpha} + \epsilon h_{,\alpha} \delta_{iz} \ , \tag{41}$$

$$\boldsymbol{e}_i \cdot \boldsymbol{n} = \delta_{iz} - \epsilon h_{,\alpha} \delta_{i\alpha} \ . \tag{42}$$

We then find the in-plane components up to linear order in $\epsilon$ to be

$$
\begin{aligned}
t^{\alpha}_{\pm} &= t^{\alpha}_{(0)\pm} \pm \epsilon \left( u^{z}_{(1),\alpha} + u^{\alpha}_{(1),z} + 2h_{,\alpha} u^{z}_{(0),z} - h_{,\beta}(u^{\beta}_{(0),\alpha} + u^{\alpha}_{(0),\beta}) \right) \ , \\
t^{\alpha}_{\pm} &= t^{\alpha}_{(0),\pm} + \epsilon t^{\alpha}_{(1),\pm} \ ,
\end{aligned}
\tag{43}
$$

and the normal components up to the same order are

$$
\begin{aligned}
t^{n}_{\pm} &= t^{n}_{(0),\pm} + \epsilon \left( 2u^{z}_{(1),z} - 2h_{,\alpha}(u^{\alpha}_{(1),z} + u^{z}_{(1),\alpha}) - p_{(1)} \right) \ , \\
t^{n}_{\pm} &= t^{n}_{(0),\pm} + \epsilon t^{n}_{(1),\pm} \ .
\end{aligned}
\tag{44}
$$

We then find the jumps and averages of the perturbed surface traction components

$$
\left[\left[ t^{\alpha}_{(1)} \right]\right] = 2 \left( \left\langle u^{z}_{(1),\alpha} \right\rangle + \left\langle u^{\alpha}_{(1),z} \right\rangle + 2h_{,\alpha} \left\langle u^{z}_{(0),z} \right\rangle - h_{,\beta} \left\langle u^{\beta}_{(0),\alpha} + u^{\alpha}_{(0),\beta} \right\rangle \right) \ , \tag{45}
$$

$$
2 \left\langle t^{\alpha}_{(1)} \right\rangle = \left( \left[\left[ u^{z}_{(1),\alpha} \right]\right] + [[ u_{(1)} z^{\alpha} ]] + 2h_{,\alpha} \left[\left[ u^{z}_{(0),z} \right]\right] - h_{,\beta} \left[\left[ u^{\beta}_{(0),\alpha} + u^{\alpha}_{(0),\beta} \right]\right] \right) \ , \tag{46}
$$

$$
\left[\left[ t^{n}_{(1)} \right]\right] = \left( 2 \left[\left[ u^{z}_{(1),z} \right]\right] - 2h_{,\alpha} \left[\left[ u^{\alpha}_{(1),z} + u^{z}_{(1),\alpha} \right]\right] - [[ p_{(1)} ]] \right) \ , \tag{47}
$$

$$
\left\langle t^{n}_{(1)} \right\rangle = \left( 2 \left\langle u^{z}_{(1),z} \right\rangle - 2h_{,\alpha} \left\langle u^{\alpha}_{(0),z} + u^{z}_{(0),\alpha} \right\rangle - \langle p_{(1)} \rangle \right) \ . \tag{48}
$$

Now, the $\mathcal{O}(\epsilon)$ equations for the in-plane and shape equations in Eqs. (18a) and (18b) become, respectively,

$$
\begin{aligned}
0 = &\lambda_{(1),\alpha} + \frac{\mathrm{SL}}{\Gamma} v^{\alpha}_{(1),\beta\beta} + \mathrm{Ca} \Big( \delta \Big( h_{,\alpha\lambda} - \delta^{\alpha}_{\lambda} \Delta_s h \Big) \left\langle u^{z}_{(0),\lambda} + u^{\lambda}_{(0),z} \right\rangle - \ell \left\langle p_{(1)} \right\rangle^{,\alpha} \Big) \\
&+ \Big( \left[\left[ u^{z}_{(1),\alpha} \right]\right] + \left[\left[ u^{\alpha}_{(1),z} \right]\right] + 2h_{,\alpha} \left[\left[ u^{z}_{(0),z} \right]\right] - h_{,\beta} \left[\left[ u^{\beta}_{(0),\alpha} + u^{\alpha}_{(0),\beta} \right]\right] \Big) \ ,
\end{aligned}
\tag{49}
$$

and

$$
\begin{aligned}
0 = &\Delta_s h \left( \lambda_{(0)} + \ell \mathrm{Ca} \left\langle u^{z}_{(0),z} \right\rangle \right) - \frac{1}{2\Gamma} \Delta^2_s h + \frac{\mathrm{SL}}{\Gamma} h_{,\alpha\beta} \left( v^{\alpha}_{(0),\beta} + v^{\beta}_{(0),\alpha} \right) + \mathrm{Ca} \left( - [[ p_{(1)} ]] \right. \\
&+ \ell \Big( \left\langle u^{z}_{(1),\alpha} \right\rangle_{,\alpha} + \left\langle u^{\alpha}_{(1),z} \right\rangle_{,\alpha} + 2h_{,\alpha\alpha} \left\langle u^{z}_{(0),z} \right\rangle + 2h_{,\alpha} \left\langle u^{z}_{(0),z} \right\rangle_{,\alpha} \\
&- h_{,\beta\alpha} \left\langle u^{\beta}_{(0),\alpha} + u^{\alpha}_{(0),\beta} \right\rangle - h_{,\beta} \left\langle u^{\beta}_{(0),\alpha} + u^{\alpha}_{(0),\beta} \right\rangle_{,\alpha} \Big) \\
&\left. + \left( 2 \left[\left[ u^{z}_{(1),z} \right]\right] - 2h_{,\alpha} \left[\left[ u^{\alpha}_{(0),z} + u^{z}_{(0),\alpha} \right]\right] \right) \right) \ .
\end{aligned}
\tag{50}
$$

Finally, the bulk perturbed continuity equation reads

$$
u^{i}_{(1),i} = 0 \ , \tag{51}
$$

and the Stokes equations are,

$$
0 = -p_{(1),i} + u^{i}_{(1),jj} \ . \tag{52}
$$

# 5 Problem solution

In this section, we solve the linear response problem outlined in the main text. First, the base state results are written down. Then, the perturbed equations from the previous section are solved using no-slip boundary conditions at the membrane-fluid interfaces and far-field conditions for the perturbations.

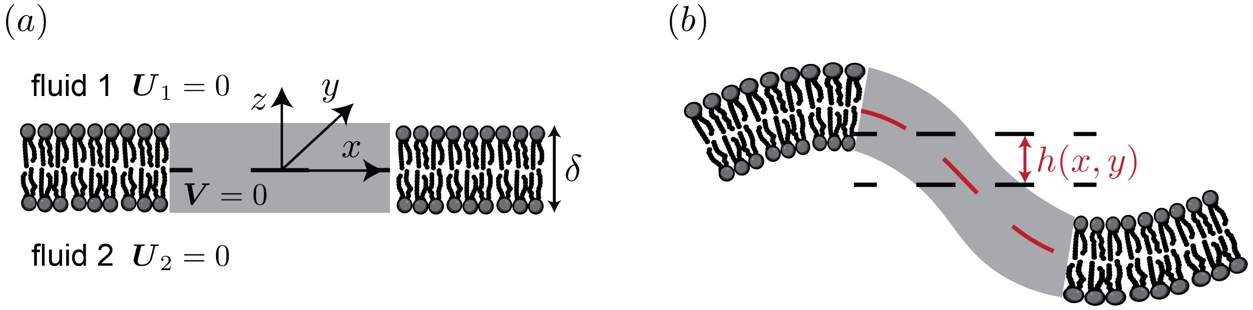


Figure 4: (a) The unperturbed membrane state. (b) The perturbed state with height field $h(x, y)$.

### 5.1 Membrane parametrization and base state

We assume the base state mid-surface takes the form of Eq. (19) from Section 4.1. Given this assumption and Eqs. (32) and (33), the 'base' state conditions for the velocities from Eqs. (21) and (24) , the bulk fluid pressure $p$, and the membrane tension $\lambda$ read

$$\boldsymbol{u}_{(0)} = 0 \ , \quad \boldsymbol{v}_{(0)} = 0 \ , \quad p_{(0)} = 0 \ , \quad \lambda_{(0)} = 1 \ , \tag{53}$$

Where the membrane tension for a homogeneous membrane is assumed to be constant. Though in Sec. 4.2 we associated perturbed quantities with the subscript (1), we will forgo this notation in the following section for clarity.

### 5.2 The perturbed equations

Given the assumed base state in Sec. 5.1, we linearize the equations about this equilibrium as in Sec. 4.2, yielding the membrane equations

$$0 = \lambda_{,\alpha} + \frac{\mathrm{SL}}{\Gamma}\Delta_s v^\alpha + \mathrm{Ca}\left[\!\left[u^\alpha_{,z} + u^z_{,\alpha}\right]\!\right] \ , \tag{54a}$$

$$0 = \Delta_s h - \frac{1}{2\Gamma}\Delta_s^2 h + \mathrm{Ca}\left(\frac{1}{2}\ell\left\langle u^\alpha_{,z\alpha} + u^z_{,\alpha\alpha}\right\rangle - [\![p]\!] + 2\left[\!\left[u^z_{,z}\right]\!\right]\right) \ , \tag{54b}$$

$$0 = v^\alpha_{,\alpha} \ , \tag{54c}$$

where $\Delta_s \equiv \partial_x^2 + \partial_y^2$, and we used that $2H \simeq \Delta_s h$. Eqs. (52) and (54c) correspond to Eqs. (2a)–(2c) in the main text.

We use the method of domain perturbations to extrapolate the quantities evaluated at $z = \pm\ell/2 + \epsilon h$ in terms of the same quantities evaluated at $z = \pm\ell/2$. In particular, the velocities and pressure become

$$u^i_\pm = u^i_\pm\Big|_{z=\pm\ell/2} + \left(\frac{\partial u^i_\pm}{\partial z}\right)_{z=\ell/2} \epsilon h + O(\epsilon^2) \ , \tag{55a}$$

$$p_\pm = p_\pm\Big|_{z=\pm\ell/2} + \left(\frac{\partial p_\pm}{\partial z}\right)_{z=\pm\ell/2} \epsilon h + O(\epsilon^2) \ , \tag{55b}$$

where, after substituting the perturbation expansion, we find that only the first terms on the right-hand side remain.

### 5.3 Linear response solution for finite thickness membranes

To proceed with the solution of Eqs. (51), (52) and (54), we exploit translation invariance of the linear operators in the $x$- and $y$-directions and decompose the unknowns into plane waves as

$$\boldsymbol{u}_{\pm}(x,y,z,t) = \sum_{q} \boldsymbol{u}_{\boldsymbol{q}\pm}(z) e^{i\boldsymbol{q}\cdot\boldsymbol{x}+\omega t} \ , \tag{56a}$$

$$p_{\pm}(x,y,z,t) = \sum_{q} p_{\boldsymbol{q}\pm}(z) e^{i\boldsymbol{q}\cdot\boldsymbol{x}+\omega t} \ , \tag{56b}$$

$$\boldsymbol{v}(x,y,t) = \sum_{q} \boldsymbol{v}_{\boldsymbol{q}} e^{i\boldsymbol{q}\cdot\boldsymbol{x}+\omega t} \ , \tag{56c}$$

$$\lambda(x,y,t) = \sum_{q} \lambda_{\boldsymbol{q}} e^{i\boldsymbol{q}\cdot\boldsymbol{x}+\omega t} \ , \tag{56d}$$

$$h(x,y,t) = \sum_{q} h_{\boldsymbol{q}} e^{i\boldsymbol{q}\cdot\boldsymbol{x}+\omega t} \ , \tag{56e}$$

where $\boldsymbol{q}\cdot\boldsymbol{x} \equiv q_x x + q_y y$, and $\omega(q)$ is the dispersion relation that encodes the relaxation dynamics of the modes. Using the ansatz of Eq. (56) in the bulk equations yields,

$$0 = \ -iq_\alpha p_{\boldsymbol{q}\pm} + (\partial_z^2 - q^2) u^\alpha_{\boldsymbol{q}\pm} \ , \tag{57a}$$

$$0 = \ -\partial_z p_{\boldsymbol{q}\pm} + (\partial_z^2 - q^2) u^z_{\boldsymbol{q}\pm} \ , \tag{57b}$$

$$0 = \ \partial_z u^z_{\boldsymbol{q}\pm} + iq_\alpha u^\alpha_{\boldsymbol{q}\pm} \ , \tag{57c}$$

with $q^2 \equiv q_x^2 + q_y^2$. Similarly, the membrane equations Eqs. (54a)–(54c) become

$$0 = iq_\alpha \lambda_{\boldsymbol{q}} - q^2 \frac{\mathrm{SL}}{\Gamma} v^\alpha_{\boldsymbol{q}} + \mathrm{Ca}\left( [\![ u^\alpha_{\boldsymbol{q},z} + iq_\alpha u^z_{\boldsymbol{q}} ]\!] \right) \ , \tag{58a}$$

$$0 = q^2 h_{\boldsymbol{q}} + \frac{1}{2\Gamma} q^4 h_{\boldsymbol{q}} - \mathrm{Ca}\left( \frac{1}{2}\ell \left\langle iq_\alpha u^\alpha_{\boldsymbol{q},z} - q^2 u^z_{\boldsymbol{q}} \right\rangle - [\![ p_{\boldsymbol{q}} ]\!] + 2\, [\![ u^z_{\boldsymbol{q},z} ]\!] \right) \ , \tag{58b}$$

$$0 = iq_\alpha v^\alpha_{\boldsymbol{q}} \ . \tag{58c}$$

We now proceed with the general solution for the bulk fluid unknowns.

We start by multiplying the in-plane equations Eq. (57a) by $iq_\alpha$ and subsequently substituting $iq_\alpha u^\alpha_{\boldsymbol{q}\pm}$ via Eq. (57c) to arrive at the following relation between the bulk pressure and $z$-velocity,

$$0 = q^2 p_{\boldsymbol{q}\pm} - (\partial_z^2 - q^2)\partial_z u^z_{\boldsymbol{q}\pm} \ . \tag{59}$$

We then derive a pressure equation by first differentiating Eq. (57b) with respect to $z$ and then substituting Eq. (59), resulting in,

$$\partial_z^2 p_{\boldsymbol{q}\pm} - q^2 p_{\boldsymbol{q}\pm} = 0 \ , \tag{60}$$

whose solution is,

$$p_{\boldsymbol{q}\pm} = P_\pm e^{\mp qz} \ , \tag{61}$$

where we have used Eq. (15b). The pressure solution of Eq. (61) is then introduced into the momentum equations, Eqs. (57a) and (57b), from which the velocity solutions are found,

$$u^z_{\boldsymbol{q}\pm} = \left( U_\pm + P_\pm \frac{z}{2} \right) e^{q\mp z} \ , \tag{62a}$$

$$u^\alpha_{\boldsymbol{q}\pm} = \left( V^\alpha_\pm \mp P_\pm \frac{q_\alpha z}{2q} \right) e^{q \mp z} \ , \tag{62b}$$

where we have used Eq. (15a).

We now turn our attention to the coupling conditions at the membrane boundaries to determine the coefficients $U_\pm$ and $P_\pm$. Using the bulk solutions in Eqs. (61), (62a) and (62b) and the no-slip conditions, Eqs. (16a) and (16b), we obtain

$$\left( U_\pm \pm P_\pm \frac{\ell}{4} \right) e^{-q\ell/2} = \omega h_{\boldsymbol{q}} \ , \tag{63a}$$

$$\left( V^\alpha_\pm - P_\pm \frac{q_\alpha \ell}{4q} \right) e^{-q\ell/2} = v^\alpha_{\boldsymbol{q}} \mp i q_\alpha \omega \frac{\ell}{2} h_{\boldsymbol{q}} \ . \tag{63b}$$

Combining the in-plane conditions in Eq. (63b) with the bulk continuity equation, Eq. (57c), and Eq. (62a), we find

$$\frac{1}{4} e^{-q\ell/2} \left( 4qU_\pm \pm P_\pm (q\ell - 2) \right) = \frac{\ell}{2} q^2 \omega h_{\boldsymbol{q}} \ . \tag{64}$$

We then use Eqs. (63a) and (64) to eliminate $U_\pm$, yielding

$$\frac{q\ell - 2}{4q} (P_+ + P_-) + \frac{\ell}{2} (P_+ + P_-) = 0 \ , \tag{65}$$

implying that for arbitrary $q$,

$$P_+ = -P_- = P \ . \tag{66}$$

Substituting this result back into the $z$-velocity conditions, Eqs. (63a) and (64), we solve for the pressure coefficient as,

$$P = \omega h_{\boldsymbol{q}} q \left( 2 - \ell q \right) e^{q\ell/2} \ . \tag{67}$$

Using Eq. (67) in Eqs. (63a) and (64) allows us to solve for the $z$-direction velocity coefficients,

$$U_+ = U_- = \frac{1}{4} \omega h_{\boldsymbol{q}} \left( 4 + q\ell(q\ell - 2) \right) e^{q\ell/2} \ . \tag{68}$$

We now turn our attention to the in-plane equations, Eq. (58a). Using the results of Eqs. (63a), (63b) and (67), Eq. (58a) reduces to

$$0 = i q_\alpha \lambda_{\boldsymbol{q}} - q \left( \frac{\mathrm{SL}}{\Gamma} q + 2\mathrm{Ca} \right) v^\alpha_{\boldsymbol{q}} \ . \tag{69}$$

Along with the membrane continuity equation in Eq. (58c), Eq. (69) implies that for arbitrary wavenumbers,

$$v^\alpha_{\boldsymbol{q}} = 0 \ , \tag{70}$$

$$\lambda_{\boldsymbol{q}} = 0 \ . \tag{71}$$

Physically, this means that perturbations do not induce in-plane lipid flow or changes in surface tension at leading order; the membrane responds purely through out-of-plane (bending) modes.

Equations (67) and (70) are then plugged into Eq. (63b), and the result is used to solve for the bulk $x$- and $y$-velocity coefficients,

$$V_+^\alpha = -V_-^\alpha = -\frac{1}{4} i\omega\ell^2 h_{\boldsymbol{q}} q q_\alpha e^{q\ell/2} \ . \tag{72}$$

Finally, we use Eqs. (67), (68) and (72) in Eq. (58b) to find the following expression for the dispersion relation $\omega$,

$$\omega(q) = -\frac{\frac{1}{2}q^4 + \Gamma q^2}{\mathrm{Ca}\Gamma q\left(4 + q^2\ell^2\right)} \ . \tag{73}$$

In summary, we obtained the non-zero real-space solutions

$$u_\pm^z(x,y,z,t) = \frac{1}{4}\sum_q \omega(q) h_{\boldsymbol{q}} \left(4 + q(\ell \mp 2z)(q\ell - 2)\right) e^{q\left(\frac{\ell}{2}\mp z\right)} e^{(i\boldsymbol{q}\cdot\boldsymbol{x} + \omega t)} \ , \tag{74}$$

$$u_\pm^\alpha(x,y,z,t) = \frac{1}{4}\sum_q \omega(q) h_{\boldsymbol{q}} i q_\alpha \left(2z(q\ell - 2) \mp q\ell^2\right) e^{q\left(\frac{\ell}{2}\mp z\right)} e^{(i\boldsymbol{q}\cdot\boldsymbol{x} + \omega t)} \ , \tag{75}$$

$$p_\pm(x,y,z,t) = \pm\sum_q \omega(q) h_{\boldsymbol{q}} q \left(2 - q\ell\right) e^{q\left(\frac{\ell}{2}\mp z\right)} e^{(i\boldsymbol{q}\cdot\boldsymbol{x} + \omega t)} \ , \tag{76}$$

$$v_m^\alpha(x,y,z,t) = -z\sum_q \omega(q) h_{\boldsymbol{q}} i q_\alpha e^{(i\boldsymbol{q}\cdot\boldsymbol{x} + \omega t)} \ , \tag{77}$$

$$v^z(x,y,t) = \sum_q \omega(q) h_{\boldsymbol{q}} e^{(i\boldsymbol{q}\cdot\boldsymbol{x} + \omega t)} \ , \tag{78}$$

where we use $v_m^\alpha$ is the total in-plane membrane velocity (including base and perturbed states), reconstructed using Eq. (4), and $\omega(q)$ is given by Eq. (73).

## 6 Dispersion relation and hydrodynamics

In this section, we analyze the linear response of a lipid membrane immersed in an incompressible Newtonian fluid, subject to shape fluctuations using the equations derived in Section 5. The goal is to explore how finite-thickness effects influence the hydrodynamics and energy dissipation of the system.

We first focus on the dispersion relation $\omega(q)$, describing how bending, tension, and finite-thickness contributions govern the relaxation dynamics of membrane fluctuations. This includes transitions between regimes dominated by tension, bending, or thickness effects, which are marked by characteristic wavenumbers ($q_1$ and $q_2$).

Next, we investigate the flow fields induced by these fluctuations at different length scales. By resolving profiles at scales both larger and comparable to the membrane thickness, we reveal how finite-thickness effects significantly alter relaxation dynamics in the thickness-dominated regime. These findings connect directly to phenomena such as pressure inversion, flow reversals, and stagnation points, as discussed in the main text.

### 6.1 Dispersion relation

The dispersion relation $\omega(q)$ (Eq. (73) and Eq. (3) in the main text) reflects how different physical mechanisms dominate membrane relaxation depending on the wavenumber. As reviewed in the

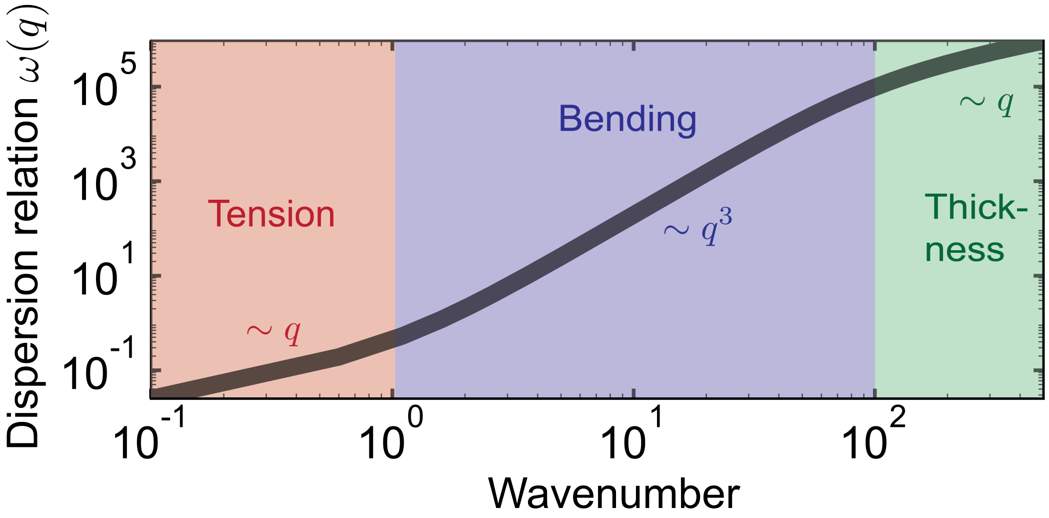


Figure 5: Dispersion relation as a function of wavenumber $q$, reproduced from Fig. 1 (b) in the main text. This highlights the transition between tension, bending, and thickness-dominated regimes.

main text, tension dominates at low $q$, bending at intermediate $q$, and finite-thickness effects at high $q$, the latter captured by the $(q\ell)^2$ correction in the denominator of $\omega(q)$.

The $q^3$-dependence emerges from hydrodynamic interactions between the bulk fluid and the membrane [16, 17]. Specifically, the term $\ell \, [\![t^{\alpha}_{visc}]\!]_{:\alpha} /2$ represents the moment resulting from shear force differences on the membrane's top and bottom boundaries. This moment, unique to finite-thickness membranes, modifies the Green's function [16, 17] governing the system's response to thermal fluctuations.

In the two-dimensional limit ($\ell \to 0$), the drag force is encoded by $1/\zeta_{\mathbf{q}} = 1/4\Gamma q$, which corresponds to the Fourier transform of the Oseen tensor for a two-dimensional membrane [16–18]. In this case, the membrane behaves as a collection of independent points, each experiencing drag as it relaxes to its flat state. For finite-thickness membranes, however, the system can be understood as a collection of rods. These rods not only relax their midpoints relative to $z = 0$ but also experience an additional rotational drag as they align with their equilibrium state. This rotational resistance introduces the $(q\ell)^2$ term in the denominator of $\omega(q)$, which dominates dissipation for $q > q_2$, as illustrated in Fig. 5. This additional dissipation mechanism highlights the importance of finite-thickness effects, especially at high wavenumbers where classical two-dimensional models fail to capture the system's full hydrodynamic complexity.

### 6.2 Induced flow fields for single modes

To gain a deeper understanding of the emergent hydrodynamic phenomena, we analyze the induced flow fields in the tension, bending, and thickness regimes. While we provide here the general solutions, we reserve discussion of the thickness regime for the main text. Instead, our primary goal is to identify and characterize the physical mechanisms responsible for the observed finite-thickness effects on the hydrodynamics of the membrane and bulk fluid.

To understand the response of the system to single-mode fluctuations, we specialize Eqs. (74) and (78) by choosing the initial height perturbation as,

$$h(x, y, z, 0) = h_0 \sin(q^* x) \ , \tag{79}$$

for the single mode $q^*$ with $h_0 = 10^{-2}\ell$. The Fourier transform of Eq. (79) leads to the following form of $h_{\boldsymbol{q}}$,

$$h_{\mathbf{q}} = h_0 \frac{1}{2i} \left(\delta(q_x - q^*) + \delta(q_x + q^*)\right) \delta(q_y). \tag{80}$$

Substituting this result into Eqs. (74) and (78) results in,

$$u^z_{\pm}(x, y, z, t) = \frac{1}{4}\omega h_0 \left(4 + q^*(\ell \mp 2z)(q^*\ell - 2)\right) e^{q^*\left(\frac{\ell}{2} \mp z\right)} e^{\omega t} \sin(q^* x) \ , \tag{81}$$

$$u^\alpha_{\pm}(x, y, z, t) = \frac{1}{4}\omega h_0 q^* \left(2z(q^*\ell - 2) \mp q^*\ell^2\right) e^{q^*\left(\frac{\ell}{2} \mp z\right)} e^{\omega t} \cos(q^* x) \ , \tag{82}$$

$$p_{\pm}(x, y, z, t) = \pm\omega h_0 q^* \left(2 - q^*\ell\right) e^{q^*\left(\frac{\ell}{2} \mp z\right)} e^{\omega t} \sin(q^* x) \ , \tag{83}$$

$$v^\alpha_m(x, y, z, t) = -z\omega h_0 q^* e^{\omega t} \cos(q^* x) \ , \tag{84}$$

$$v^z(x, y, t) = \omega h_0 e^{\omega t} \sin(q^* x) \ . \tag{85}$$

With Eqs. (81)–(85), we are now in a position to study the hydrodynamic response of the membrane and the bulk fluid.

### 6.2.1 Flows in the tension and bending regimes

We now present the flow field solutions for two different modes, corresponding to the tension and bending regimes, using the same physical parameters as in the *Results* section of the main text. For these parameter values, the crossover from tension to bending modes occurs at $q_1 = 1.14$. Since the time dependence is purely exponential, we focus on the flows at $t = 0$, as they qualitatively remain the same but decrease in magnitude over time. We illustrate the velocity flow fields for $\ell = 0.02$ (the $(2 + \delta)$-dimensional case) and $\ell = 0$ (the 2-dimensional case) for modes $q = 0.3 < q_1$ and $q = 30.0 < q_2$ in Figure 6, utilizing the equations solutions provided by equations Eqs. (81)–(85).

Figure 6 shows that the dominant motion at the membrane surfaces occurs in the normal direction for both theories and at both $q = 0.3$ and $q = 30.0$. Given the initial perturbation in Eq. (79), the flow maxima occur at $x = (2n + 1)\pi/2q$ where $n \in \mathbb{Z}$ and $h = \pm h_0$. Minima in the initial perturbation ($h = -h_0$) push and drag bulk fluid in the positive $z$-direction, while maxima ($h = h_0$) do so in the opposite direction. This is marked by pressure maxima and minima occurring at the height field crests and troughs, respectively. In the tension and bending regimes, pressure builds up at the height field troughs monotonically, as shown in Fig. 7, where we plot Eq. (83) at $(x = 3\pi/2q, z = \ell/2)$ as a function of wavenumber. Due to incompressibility in the bulk fluids, vortices develop about the membrane, as fluid flows from pressure maximum sources to pressure minimum sinks. In this regime, the velocity perturbations in the bulk fluid decay spatially on $\mathcal{O}(10L)$.

As we increase the perturbation frequency to the bending regime where $q_1 < q^* < q_2$, we find that the flow distributions qualitatively remain similar to the tension regime. The flow patterns remain the same, but the spatial decay length of velocity perturbations in the bulk fluid decreases significantly to be of $\mathcal{O}(0.1L)$ since this decay length is inversely proportional to the initial condition wavenumber. However, as noted in Section 6.1 and in the main text, the flow fields in the bending regime do not exhibit appreciable finite thickness effects. Rather, we gain further insight into the induced hydrodynamics by again considering the surface pressure at the trough at $(x = 3\pi/2q, z = \ell/2)$, as shown in Fig. 7. While the pressure at this trough matches in the strict two-dimensional and $(2+\delta)$-dimensional theories for lower wavenumbers, they diverge as the perturbation frequency

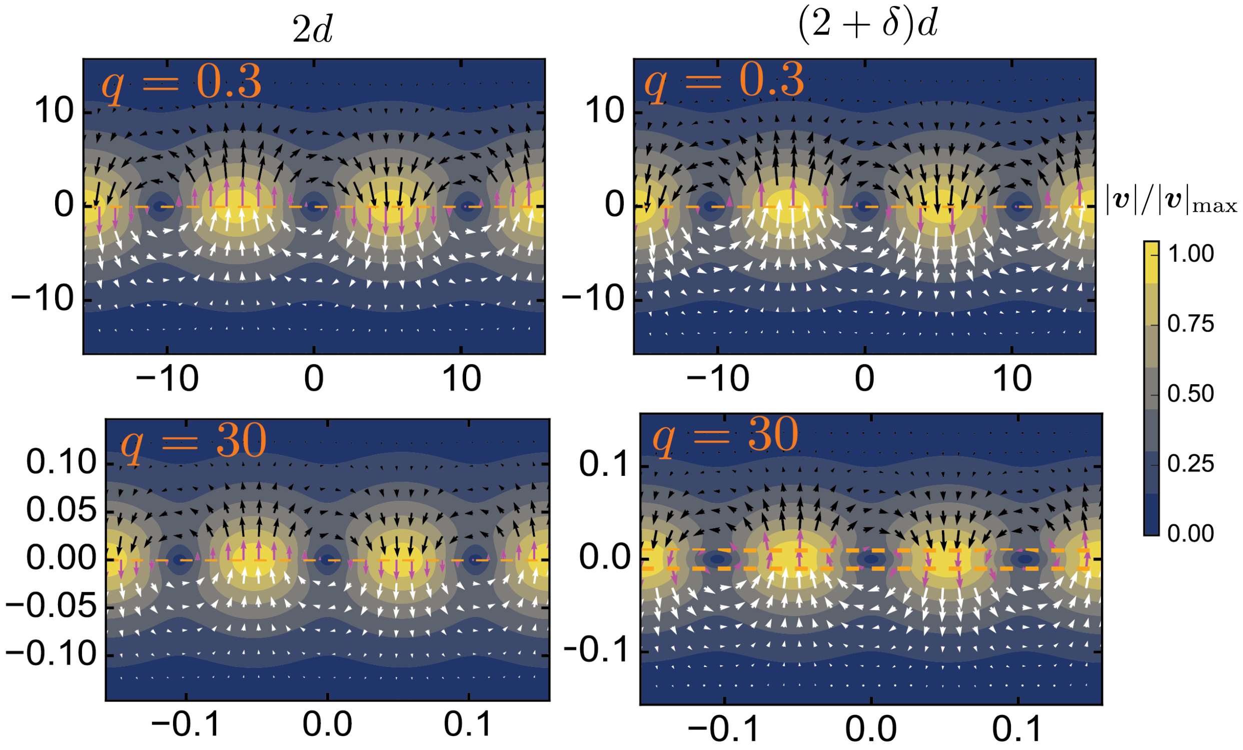


Figure 6: The normalized flow fields in the tension ($q = 0.3$) and bending ($q = 30$) regimes for the two-dimensional and $(2+\delta)$-dimensional theories. Black arrows correspond to fluid flow above the membrane, white to below the membrane, and magenta to the membrane surface motion. The orange dashed lines indicate the membrane surfaces. In all cases, the predominant surface motion is in the normal, or $z$-, direction. The flow patterns exhibit little difference, with circulations occuring about the membrane. Though the membrane thickness becomes "visible" for $q = 30$, it does not affect the induced hydrodynamics at this wavenumber.

increases deep in the bending regime. As discussed in the *Results* section of the main text, this is due to how finite thickness effects manifest in the bulk pressure.

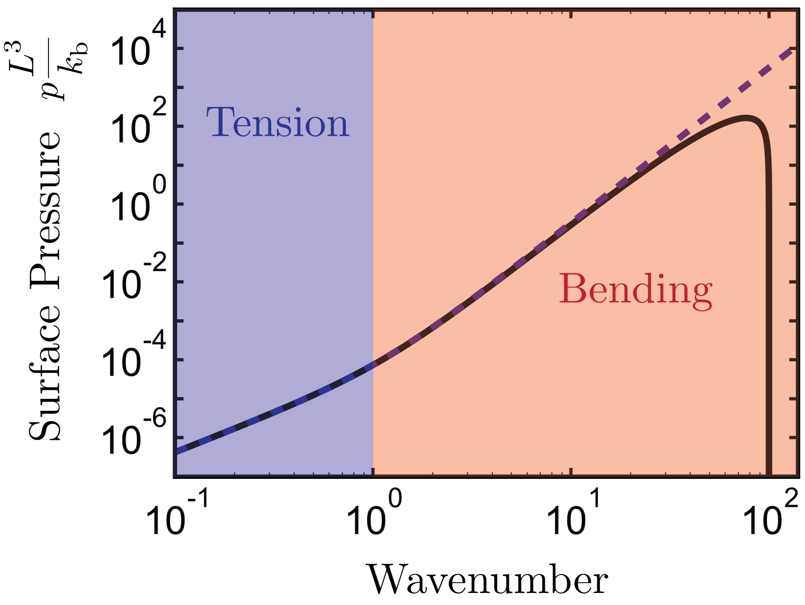


Figure 7: The maximum pressure per wavenumber $q$ for the tension and bending regimes. The dashed line corresponds to the two-dimensional result while the solid line is the $(2+\delta)$-dimensional theory. Pressure build up occurs predominantly due to bending fluctuations, indicating high-frequency modes lead to stronger circulations.

### 6.3 The emergence of flow reversal

As discussed in the *Results* section of the main text, thickness effects lead to the emergence of flow reversal and pressure inversion for high wavenumber modes. In this section, we derive the conditions for the formation of stagnation points, classify them as either vortex or extensional, and analyze their strain and rotation characteristics. We note that due to the periodic nature of the perturbation, it is sufficient to focus on two representative stagnation points in the upper half-plane. To that end, we set Eq. (81) and Eq. (82) to zero to find the following set of stagnation points,

$$(x,z)_{\text{ext}} = \left(\frac{\pi}{2q}, \frac{\ell}{2} + \frac{2}{q(\ell q - 2)}\right), \tag{86}$$

$$(x,z)_{\text{vortex}} = \left(\frac{\pi}{q}, \frac{\ell}{2} + \frac{\ell}{\ell q - 2}\right). \tag{87}$$

To characterize the flow behavior at these points, we calculate the strain rate tensor, defined as $\boldsymbol{D} = \frac{1}{2}(\nabla \boldsymbol{u} + \nabla \boldsymbol{u}^T)$, as a function of the wavenumber. We find that at $(x,z)_{\text{vortex}}$, $\boldsymbol{D} = \boldsymbol{0}$, suggesting there is no strain at the vortex stagnation points. However, at $(x,z)_{\text{ext}}$, we have

$$\boldsymbol{D}\Big|_{(x,z)_{\text{ext}}} = \begin{pmatrix} \frac{1}{2}\omega h_0 q(\ell q-2)\exp\left(\frac{-2}{\ell q-2}\right) & 0 \\ 0 & -\frac{1}{2}\omega h_0 q(\ell q-2)\exp\left(\frac{-2}{\ell q-2}\right) \end{pmatrix} = \begin{pmatrix} \dot{\epsilon} & 0 \\ 0 & -\dot{\epsilon} \end{pmatrix}, \tag{88}$$

which shows that these stagnation points are marked by extensional flows. The corresponding flow field is plotted in Fig. 8–(b).

To further understand the nature of the stagnation points, we consider the rotation rate, $\boldsymbol{W} = \frac{1}{2}(\nabla \boldsymbol{u} - \nabla \boldsymbol{u}^T)$ at each type of stagnation point. At the extensional points, we find $\boldsymbol{W} = \boldsymbol{0}$,

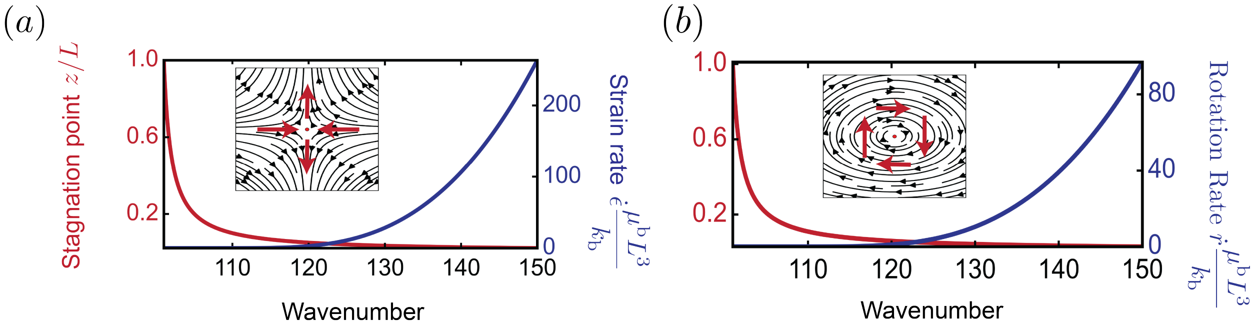


Figure 8: (a) The position of and strain rate at the stagnation point with purely extensional flow. (b) The position of and rotation rate at the stagnation point with purely circulatory flow. Both panels have insets with the streamlines about each respective stagnation point.

confirming that they are characterized by pure shear transformations due to hydrodynamic compressive and expansive forces. At the vortex points, the rotation rate reads,

$$\boldsymbol{W}\Big|_{(x,z)_{\text{vortex}}} = \begin{pmatrix} 0 & -\frac{1}{4}\omega h_0 q(\ell q-2)\exp\left(\frac{-2}{\ell q-2}\right) \\ \frac{1}{4}\omega h_0 q(\ell q-2)\exp\left(\frac{-2}{\ell q-2}\right) & 0 \end{pmatrix} = \begin{pmatrix} 0 & -\dot{r} \\ \dot{r} & 0 \end{pmatrix} . \quad (89)$$

Thus, these points exhibit pure rotation and no elongation or shear, as shown in Fig. 8, and hence, do not contribute to viscous dissipation in the bulk.

# 7 Comparison with intermonolayer slip theories

In this section, we compare our results with the intermonolayer slip (IS) model [20,21], which is the most widespread model for fluctuations of membranes at the nanoscale [22,23]. IS has been suggested as an intramembrane dissipative source to account for non-equilibrium dynamics of lipid bilayers [24] due to the finite thickness nature of the membrane. However, it is still a fundamentally two-dimensional framework. In IS, the monolayers of the bilayer are considered separate, allowing one to slip past the other, as shown in Fig. 9 (a)–(ii). To account for this, a phenomenological coefficient $b$ is introduced to couple the monolayers through a dissipative frictional force, $\boldsymbol{f}_{\text{fric}} := b(\mathbf{v}^+ - \mathbf{v}^-)$. This dynamically manifests in two dispersion relations, which we label $\text{IS}_1$ and $\text{IS}_2$ in Fig. 9 (b), encoding fast and slow modes, respectively. At high wavenumbers (e.g. $q > q_2$), the slower mode becomes constant while it can be shown that the faster mode scales with $q^3$ [20, 22]. Physically, the faster and slower modes correspond to height and density field relaxations, respectively. It can be shown that the static density difference between the two monolayers is related to the height field through $\rho_{\mathbf{q}} = dq^2 h_{\mathbf{q}}$ [25], where in this model $d$ is a measure of thickness that describes the distance between the neutral surfaces of the two layers and $\rho := \rho^+ - \rho^-$ is the difference between neutral surface densities of the top (+) and bottom (−) monolayers projected onto the surface separating the monolayers. Because the layers are physically separate and coupled only through the intermonolayer friction, such differences are permitted as each monolayer bends independently. For example, when the top monolayer experiences compression at the bilayer mid-surface, the bottom monolayer experiences expansion so that the bilayer in total undergoes bending. Because the two monolayers are compressible at the mid-surface, in-plane flows develop at the mid-surface due to continuity [19,26]. Though the mechanism is different, the IS model therefore is differentiated from

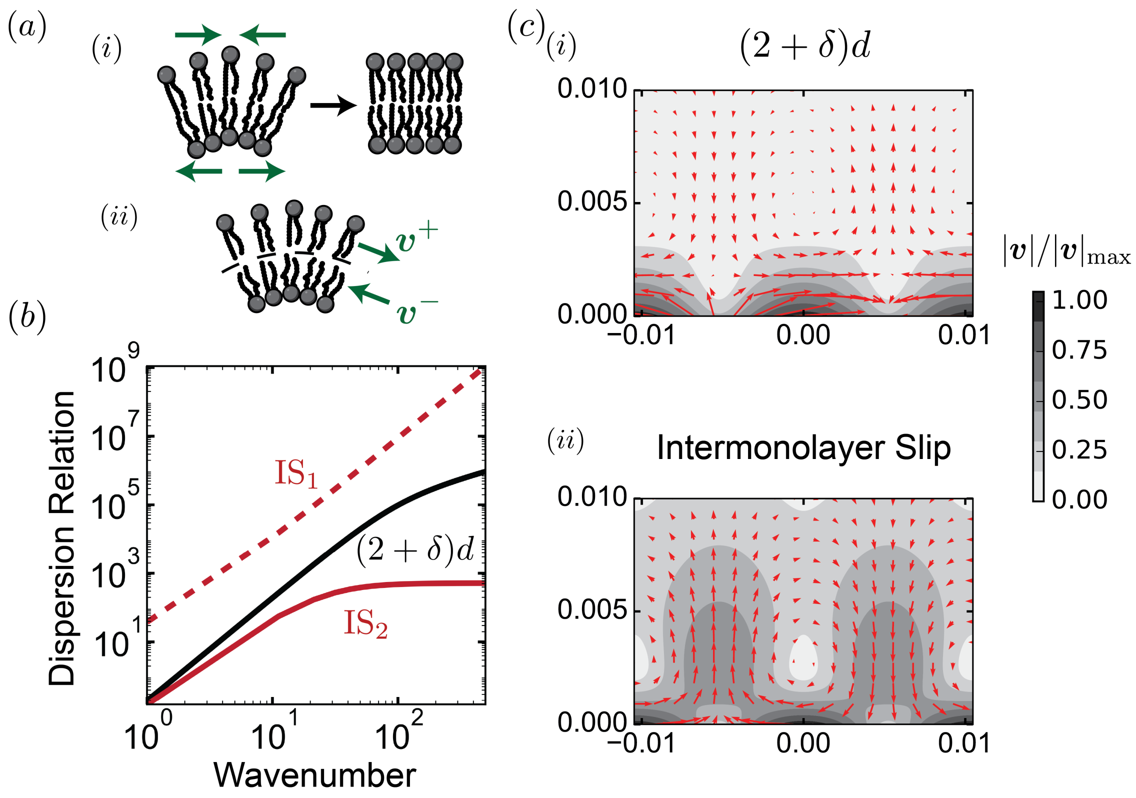


Figure 9: (a)–(i),(ii) The lipid reorientiation mechanisms proposed in this work and the IS model. (b) The dispersion relations for the IS model and the finite thickness model of the present work. In the IS model, two dispersion relations are necessary to describe the separate density and height mode dynamics. In our work, the height modes alone govern the dynamics of the bilayer. (c)–(i),(ii) Upper half-plane flow fields at $q = 300$ for the present finite thickness theory and the IS model, respectively. For comparison, we used the representative parameters $b = 10^9$ pN $\cdot$ $\mu$s/nm, $\Lambda =$ $10^-8$ pN/nm, $\mu^{\mathrm{b}} = 10^-3$ pN $\cdot$ $\mu$s/nm$^2$, $\mu^{\mathrm{m}} = 1$ pN $\cdot$ $\mu$s/nm, $\kappa = 100$ pN $\cdot$ nm, $k_{\mathrm{m}}$ 100 pN/nm [19].

strict surfaces theories in a similar manner to the $(2+\delta)$-dimensional theory in that both predict in-plane motion at the membrane surface due to thickness effects.

To study the hydrodynamic response in the bulk, one may follow the steps outlined in Ref. [19], where a Rayleighian is constructed and minimized with respect to quantities of interest to derive dynamic equations of motion, in accordance with Onsager's variational principle [27]. Figures 9 (c)–(i) & (ii) show the flow fields in the upper half plane for the $(2+\delta)$-dimensional and IS theories, respectively. Both exhibit vortex flows above the points where the height field remains zero and where we observe surface in-plane motions. However, as discussed, our theory predicts these phenomena as a result of lipid reorientations, which are three-dimensional. The IS theory treats the two monolayers as surfaces located at $z = \{0^+, 0^-\}$, whose in-plane flows are inherently two-dimensional and result from density mode relaxation. While IS introduces a phenomenological dissipative mechanism to account for intermonolayer friction, our theory effectively refines the treatment of hydrodynamic coupling at the membrane surfaces without requiring additional assumptions. In contrast to IS, we have shown here a model that allows us to capture the three-dimensional viscous-elastic nature of the lipid bilayers. It is possible that the two in unison will allow for a more complete theory for lipid bilayer dynamics across all scales.

## References


[1] Bassereau, P., Sorre, B. & Lévy, A. Bending lipid membranes: Experiments after W. Helfrich's model. *Advances in Colloid and Interface Science* **208**, 47–57 (2014). Publisher: Elsevier B.V.

[2] Tsafrir, I., Caspi, Y., Guedeau-Boudeville, M. A., Arzi, T. & Stavans, J. Budding and tubulation in highly oblate vesicles by anchored amphiphilic molecules. *Physical Review Letters* **91**, 1–4 (2003).

[3] Aris, R. *Vectors, Tensors, and the Basic Equations of Fluid Mechanics* (Dover Publications, New York City, 1989).

[4] Gurtin, M. E., Fried, E. & Anand, L. *The mechanics and thermodynamics of continua* (Cambridge university press, 2010).

[5] Omar, Y. A., Lipel, Z. G. & Mandadapu, K. K. (2+ $\delta$)-dimensional theory of the electromechanics of lipid membranes: Electrostatics. *Physical Review E* **109**, 054401 (2024).

[6] Omar, Y. A., Lipel, Z. G. & Mandadapu, K. K. The $(2 + \delta)$-dimensional theory of the electromechanics of lipid membranes: Ii. balance laws. *arXiv preprint arXiv:2309.03863* (2023).

[7] Omar, Y. A., Lipel, Z. G. & Mandadapu, K. K. The $(2 + \delta)$-dimensional theory of the electromechanics of lipid membranes: Iii. constitutive models. *arXiv preprint arXiv:TBD* (2024).

[8] Boyd, J. P. *Chebyshev and Fourier spectral methods* (Courier Corporation, 2001).

[9] Purcell, E. M. Life at low Reynolds number. *American Journal of Physics* **45**, 3–11 (1977).

[10] Sahu, A., Glisman, A., Tchoufag, J. & Mandadapu, K. K. Geometry and dynamics of lipid membranes: The Scriven-Love number. *Physical Review E* **101**, 1–16 (2020).

[11] Alberts, B. *et al. Molecular Biology of the Cell* (Garland Science, New York City, 2002).

[12] Phillips, R. Membranes by the Numbers. *Physics of Biological Membranes* 73–105 (2018).

[13] Deen, W. M. *Analysis of Transport Phenomena* (Oxford University Press, 2011).

[14] Lidmar, J., Mirny, L. & Nelson, D. R. Virus shapes and buckling transitions in spherical shells. *Physical Review E - Statistical Physics, Plasmas, Fluids, and Related Interdisciplinary Topics* **68**, 1–10 (2003). ArXiv: cond-mat/0306741.

[15] Sahu, A., Glisman, A., Tchoufag, J. & Mandadapu, K. K. Geometry and dynamics of lipid membranes: the scriven-love number. *Physical Review E* **101**, 052401 (2020).

[16] Doi, M. & Edwards, S. F. The Theory of Polymer Dynamics-Oxford University Press (1988). Pages: 391 Place: New York City.

[17] Granek, R. From Semi-Flexible Polymers to Membranes: Anomalous Diffusion and Reptation. *Journal de Physique I* **7**, 1761–1788 (1997).

[18] Takatori, S. C. & Sahu, A. Active Contact Forces Drive Nonequilibrium Fluctuations in Membrane Vesicles. *Physical Review Letters* **124**, 158102 (2020).

[19] Fournier, J. B. On the hydrodynamics of bilayer membranes. *International Journal of Non-Linear Mechanics* **75**, 67–76 (2015). Publisher: Elsevier.

[20] Seifert, U. & Langer, S. A. Viscous modes of fluid bilayer membranes. *Europhysics Letters* **23**, 71–76 (1993).

[21] Evans, E. & Yeung, A. Chemistry and Physics of LIPIDS Hidden dynamics in rapid changes of bilayer shape. *Chemistry and Physics of Lipids* **73**, 39–56 (1994).

[22] Watson, M. C., Peng, Y., Zheng, Y. & Brown, F. L. The intermediate scattering function for lipid bilayer membranes: From nanometers to microns. *Journal of Chemical Physics* **135** (2011).

[23] Kelley, E. G., Frewein, M. P. K., Czakkel, O. & Nagao, M. Nanoscale Bending Dynamics in Mixed-Chain Lipid Membranes. *Symmetry* **15**, 191 (2023).

[24] Evans, E. & Yeung, A. Hidden dynamics in rapid changes of bilayer shape. *Chemistry and Physics of Lipids* **73**, 39–56 (1994).

[25] Seifert, U. Configurations of fluid membranes and vesicles. *Advances in Physics* **46**, 13–137 (1997).

[26] Rahimi, M. & Arroyo, M. Shape dynamics, lipid hydrodynamics, and the complex viscoelasticty of bilayer membranes. *Physical Review E - Statistical, Nonlinear, and Soft Matter Physics* **86**, 1–15 (2012).

[27] Doi, M. Onsager's variational principle in soft matter. *Journal of Physics Condensed Matter* **23** (2011).
